# Supplementary material for: Charge Puddles in Graphene Near the Dirac Point
Source: arXiv:1512.05304 source file (2015-12-16)
Supplement: Supplementary file 1 [file Supp_Info_puddles_light.pdf]

**Supplementary Information to**
*« Charge Puddles in Graphene Near the Dirac Point »*

S. Samaddar, I. Yudhistira, S. Adam, H. Courtois, and C. B. Winkelmann

# I Sample fabrication

The graphene in our device is single-layered and obtained by mechanical exfoliation of Kish graphite on $SiO_2$ (285 nm)/Si substrate. Prior to exfoliation, the substrates are cleaned with acetone and rinsed in IPA and eventually in RBS. Finally, they are exposed to oxygen plasma (50 W). This removes organic contaminants or hydrocarbons that usually exist on the sample surface, leaving behind negatively charged silanol groups that possess a great affinity towards carbon molecules [1]. The ensuing high surface-graphene interaction is expected to reduce the van der Waals interaction between the bottom and the successive carbon layer, thus increasing the chances of occurrence of monolayers with large dimensions.

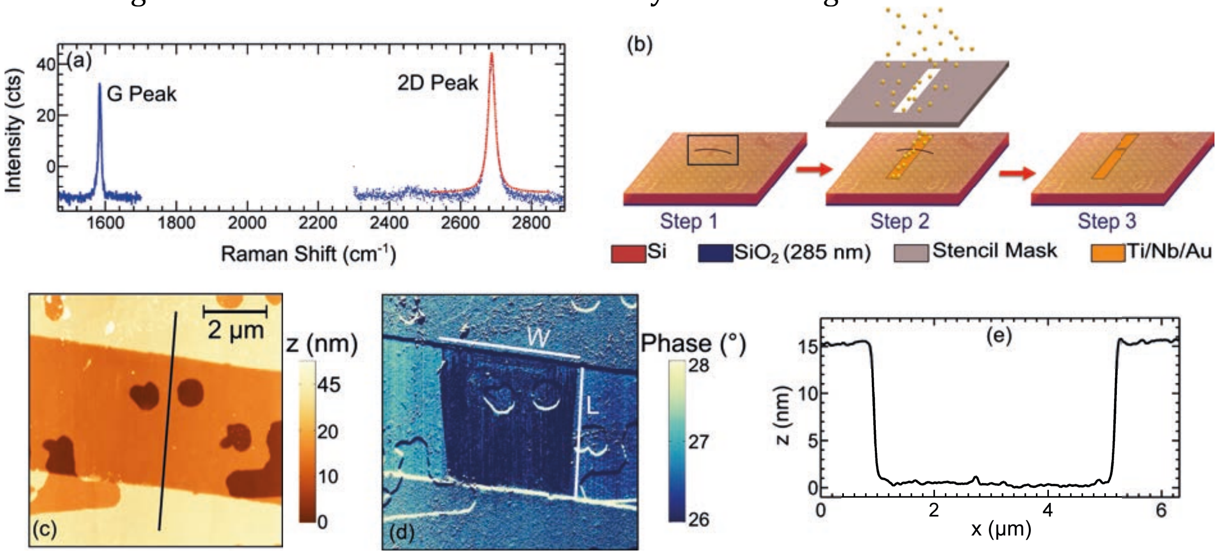


**Fig. 1S: (a)** Raman spectrum of the measured graphene flake, right after exfoliation. Red line indicates Lorentzian fit with FWHM ≈ 23 $cm^{-1}$. **(b)** Steps for positioning of mechanical masks (W wire + metallic stencil mask with rectangular slit) on the sample for depositing two isolated electrical contacts. **(c)** AFM (ex-situ, tapping mode) topography of the contacted graphene flake. **(d)** Simultaneously acquired Phase image (GR = graphene). Holes and crosses are part of the 16 bit binary code (main paper). (e) Height profile along the black line indicated in (c).

Fig. 1S(a) shows the Raman spectrum of the measured graphene flake before deposition of the metal leads. The distinct Lorentzian profile of the 2D peak with width 23 $cm^{-1}$ (full width at half maximum, FWHM) confirms the flake to be single-layered [2]. The fact that (1) the intensity ratio between the 2D peak and G peak is about $1.4 < IR_0 \approx 3$, (2) the position of the G peak is 1584 $cm^{-1} > G_0 \approx 1582$ $cm^{-1}$ and (3) width of the G peak is 7.5 $cm^{-1} < \Gamma_0^G \approx 16$ $cm^{-1}$, where ($IR_0$, $G_0$, $\Gamma_0^G$) are the respective quantities in undoped graphene, indicates that the flake was already doped before contacting. Further, the 2D position of about 2687 $cm^{-1} > 2D_0 \approx 2685$ $cm^{-1}$ where $2D_0$ is the corresponding position in the undoped case, implies that the nature of doping is p-type [3,4].

Two isolated electrical contacts (labelled *Source* and *Drain* in Fig. 1(a) of main paper) made of Ti/Nb/Au (1.5 nm/10 nm/2 nm) were fabricated using mechanical masking in order to avoid

the use of organic resists so as to ensure a clean resist-free graphene surface for the implementation of scanning probe microscopy. Fig. 1(b) illustrates the different steps involved in the fabrication process. A clean tungsten wire (about 4 μm in diameter and 0.5-0.6 mm in length) is positioned over the selected graphene flake with the help of a micro-manipulator. A second metallic mask, containing a rectangular window of size 0.3 x 2 $mm^2$ is carefully positioned on top of the flake such that the flake, with the W wire on top, is adjusted to the center of the window.

After annealing at 150°C for half an hour in UHV, the contacts are deposited, consisting of a sticking layer of titanium (1.5 nm), niobium (10 nm) capped with a thin layer of gold (2 nm) to protect against surface oxidation. The presence of niobium renders the contacts superconducting ($T_c \approx 7.1$ K) at low temperatures, which was intended for a separate study. However, in the present case, the superconducting nature of the leads has no particular significance as the scanning probe measurements were performed far (> 1 μm) from the metal-graphene interface and transport measurements were performed at large bias voltages > 5 mV.

Fig. 1S (c)-(e) show the AFM characterization of the end sample. The surface roughness (RMS) of graphene is about 0.25 nm (1 x 1 $\mu m^2$) while that of the surrounding substrate is about 0.28 nm. The height profile in (e) shows a well-defined metal-graphene interface with a step height of about 15 nm corresponding to the thickness of the metal contacts. The length of the graphene flake is L ≈ 4.3 μm while the width is about W ≈ 4.2 μm.

**II STM topographs**

Fig. 2S (a)-(e) shows STM topographs acquired on the same region at different gate voltages $V_g$, while (f)-(j) shows the simultaneously acquired DOS maps tracking the evolution of the charge puddles. The fluctuations in the DOS maps are seen to grow in size as $V_g$ approaches the Dirac point against an almost constant map of surface corrugations. The qualitatively similar topography images convincingly portray that the investigation site did not drift during the entire course of measurement. While the lateral extent of the topographic corrugations remains about 10 nm, the standard deviation characterizing the surface roughness is found to systematically increase from about 70 pm to 120 pm as $V_g$ is tuned close to charge neutrality, seen clearly in Fig. 2S (k). This apparent increase is most likely due to the influence of the LDOS in the STM topographs.

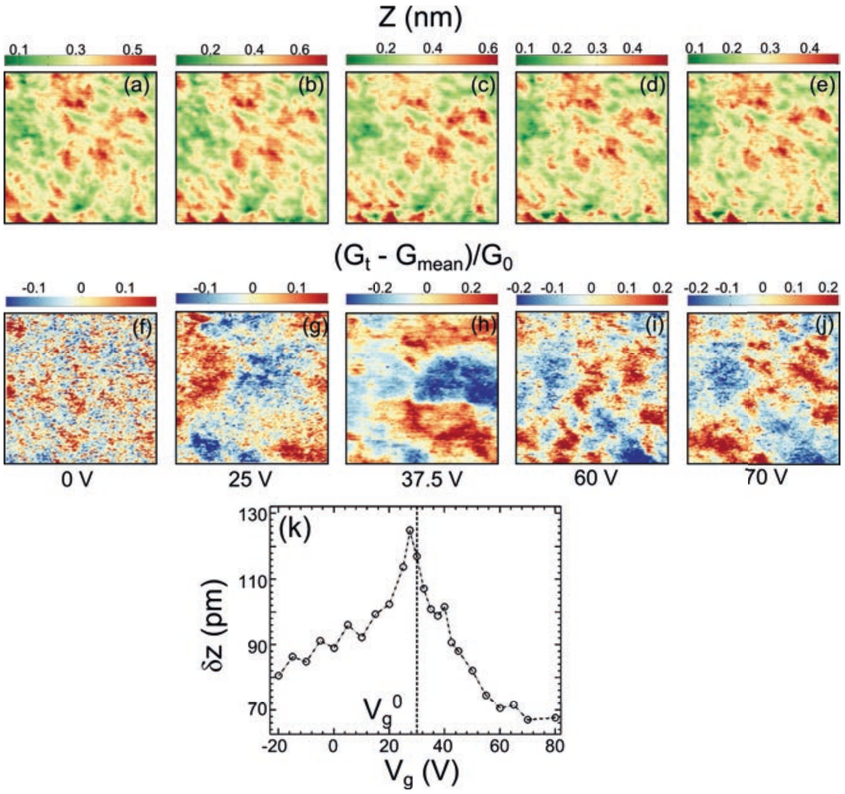


**Fig. 2S: (a)-(e)** STM topography and **(f)-(j)** simultaneously acquired normalized DOS maps $[(G_t(x,y) - \bar{G})/G_0]$ at different $V_g$ (indicated at the bottom of each column containing the Z and the corresponding DOS maps). Imaging parameters: Set-point current of $I_t$ = 50 pA and bias voltage $V_b$ of **(a, f)** 0.270 V, **(b, g)** 0.156 V, **(c, h)** -0.199 V, **(d, i)** -0.282 V and **(e, j)** -0.308 V. A modulating voltage of amplitude $V_{AC}$ = 12 mV and frequency f = 322.4 Hz was superposed on the bias voltage to acquire the DOS in **(f)-(j)**. **(k)** Surface roughness as a function of $V_g$.

## III Transport data analysis

Since the conductivity is measured in a two-probe configuration, it has contributions from the wires leading up to the sample as well as the metal-graphene contact resistances. This additional resistance $R_{series}$ is estimated by fitting the total resistance using [5]

$$R = R_{series} + \left(\frac{L}{W}\right)\frac{1}{\mu\sqrt{(n^* e)^2 + \left\{C_g\left(V_g - V_g^{\,0}\right)\right\}^2}} \quad . \qquad (1)$$

Here n* is the residual carrier concentration at charge neutrality point $V_g^0$, μ is the mobility and $C_g$ = 1.21 x $10^{-4}$ $Fm^{-2}$ is the gate capacitance per unit area corresponding to 285 nm of $SiO_2$ of the substrate with dielectric constant 3.9. μ, $R_{series}$ and $n^*$ are the fit parameters.

Due to a slight asymmetry between the electron and the hole sides, it is not possible to satisfactorily fit the data with Eq. (1) for the full range of gate voltage. However, separately fitting the hole and the electron conductivity is possible. Fig.3S (a) shows the variation of $R(V_g)$ together with the separate fits with Eq. (1) for the electron and hole sides. The extracted parameters are summarized in the following table.

| Carrier | $R_{series}$ (Ω) | $V_g^0$ (V) | μ ($cm^2V^{-1}s^{-1}$) | n* ($10^{11}$ $cm^{-2}$) | $n_i$ ($10^{11}$ $cm^{-2}$) |
|---|---|---|---|---|---|
| Electron | 400 | 29 | 5700 | 4.9 | 8.6 |
| Hole | 320 | 29 | 6400 | 4.4 | 7.6 |

**Table1S:** Summary of parameters extracted from transport. $R_{series}$ is the series resistance due to the connecting wires leading up to the sample and the metal-graphene contact resistance, $V_g^0$ is the charge neutrality point, μ is the mobility of graphene, n* is the residual carrier concentration and $n_i$ is the concentration of charge impurities in the substrate.

The best fit for $R_{series}$ for holes and electrons differs by about 20%. Work-function mismatch induced doping by the metal leads [6,7] is a possible explanation for this difference. The extracted mobilities are also found to differ, which can be attributed to the difference in scattering cross-sections off charged impurities for electrons and holes in the case of Dirac fermions [8]. The contribution of $R_{series}$ is then subtracted from the total resistance to get the conductivity of graphene. This has been shown in Fig.4S (b) [blue curve]. The linear variation with carrier concentration suggests scattering from charged impurities in the substrate to be the dominant scattering mechanism affecting carrier transport in the device [9].

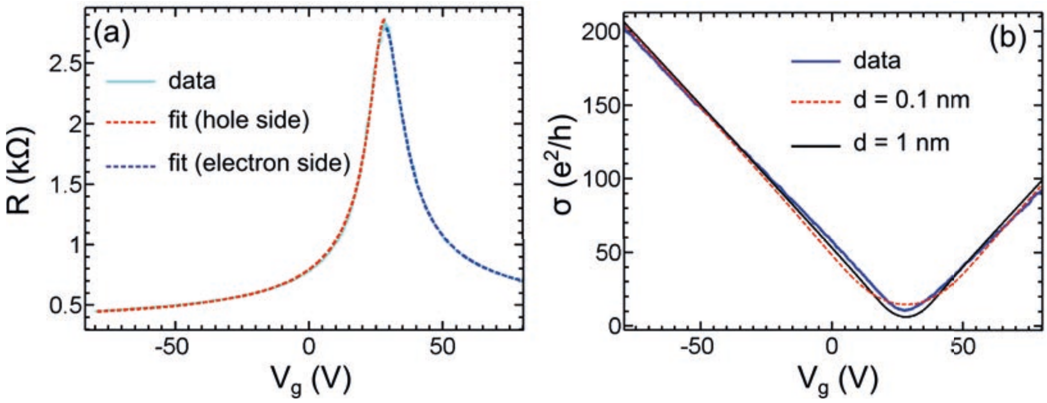


**Fig. 3S: (a)** Variation of the total two-probe resistance with back-gate voltage along with the individual fits with Eq. (1) for electron and hole sides. **(b)** Conductivity (blue line), after subtracting out the contribution of the series resistance, as a function of $V_g$. The black and red lines give the fits with Effective Medium Theory (EMT) [10]. The black line corresponds to fit parameters $n_i$ = 75 x $10^{10}$ $cm^{-2}$ and d = 1 nm while the black dashed line is calculated with same $n_i$ but d = 0.1 nm.

Using the RPA-Boltzmann formalism [9], the mobility of the device can be related to the concentration of charged impurities in the substrate using

$$n_i = 20\left(\frac{e}{h}\right)\frac{1}{\mu} \quad . \qquad (2)$$

We now focus on the behavior near charge neutrality. The experimentally obtained conductivity shows good agreement with that derived from the Effective Medium theory (EMT) [10], which is able to describe the full crossover from the regime of high to low carrier density. Fig. 3S (b) shows the measurements together with the theoretically calculated conductivities (black solid and red dashed lines) for $n_i$ = 7.5 x $10^{11}$ $cm^{-2}$ (Table 1S, hole side) for two different values of impurity distances *d* = 1 nm and 0.1 nm, assuming a Gaussian distribution of carrier concentration at all $V_g$. Such a range of *d* is typical for $SiO_2$/Si substrate [9,11].

## IV Local Gating by the tip

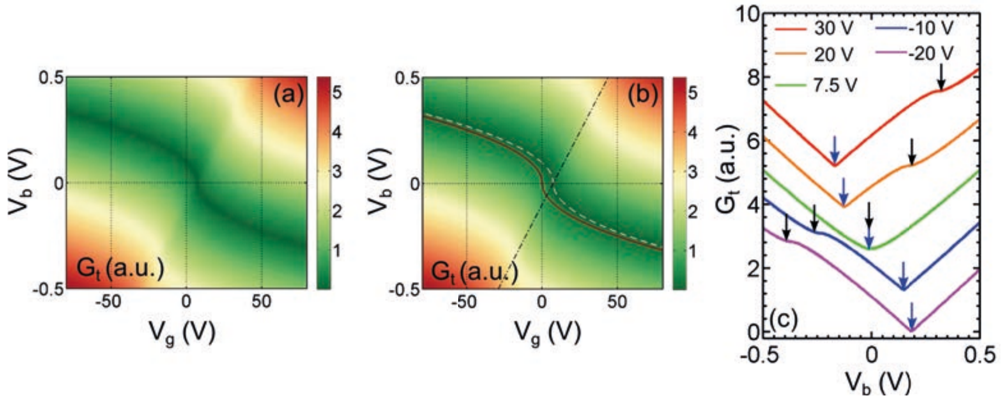


**Fig. 4S**: **(a)** Simulation of differential tunneling conductance $G_t$ to graphene at T = 0 K considering gating effect of the tip [Eq. (3), Δ = -0.1 V, $z_{ts}$ = 1 nm]. **(b)** Same as in **(a)** but with calculated values of $E_D$ ($V_g^0$ = 29 V, brown curve), primary minimum $V_b^0$ [Eq. (8), white dashed curve] and secondary minimum $V_b'$ [Eq. (8), black dashed curve] superposed. (c) Calculated $G_t$ as a function of $V_b$ at different Vg. Blue and black arrows indicate the position of $V_b^0$ and $V_b'$ respectively.

Since the differential tunneling conductance $G_t$ on graphene at T = 0 K is proportional to the DOS, we have [12]

$$G_t\left(V_b, T = 0K\right) \propto \rho\left(E = eV_b\right) = \frac{2}{\pi h^2 v_F^{\ 2}}\left|eV_b - E_D\right| \quad , \tag{3}$$

where ρ(E) is the DOS of single-layered graphene [13], h is the Planck constant and $v_F$ = 1.1 x $10^6$ $ms^{-1}$ is the Fermi velocity of graphene [14].

Due to the work-function mismatch between the tip and the sample, the potential difference between them will not be zero when they are electrically connected but will be equal to their contact potential difference $V_{CPD}$. Consequently, when a bias voltage is applied to the graphene $V_b$, the effective potential difference between them is $V_b$ - $V_{CPD}$. Therefore, the total carrier density induced in graphene due to the gating effect of the metallic tip and the back-gate

$$n = \frac{K\varepsilon_0}{et}\left[V_g - \beta\left(V_b - V_{CPD}\right)\right] \tag{4}$$

where $\beta = t/Kz_{ts}$, t = 285 nm is the gate oxide thickness in the substrate, K = 3.9 is its dielectric constant and $z_{ts}$ is the tip-sample distance.

With a change in $V_g$, $V_{CPD}$ varies due to the change in graphene work-function which is described by the following equation [15].

$$V_{CPD} = \frac{\Delta + E_D}{e} \quad , \tag{5}$$

where Δ is the work function difference between charge neutral graphene and tip.

Therefore, using n = $4\pi(E_D/hv_F)^2$ and (4), the local Dirac point due to the combined action of the tip and the back-gate will be given by

$$E_D = -\gamma e \,\mathrm{sign}\left[V_g - \beta\left(V_b - (\Delta + E_D)/e\right)\right]\sqrt{\left|V_g - \beta\left(V_b - (\Delta + E_D)/e\right)\right|} \tag{6}$$

where $\gamma = \hbar v_F \sqrt{\frac{\pi K \epsilon_0}{e^3 t}} = 0.032\ V^{1/2}$.

Solving the above second order equation for $E_D$ gives the following solution.

$$E_D = -\frac{\gamma e}{2}\,\mathrm{sign}(\nu)\left(-\beta\gamma + \sqrt{4|\nu| + \beta^2\gamma^2}\right) \qquad (7)$$

where

$$\nu = V_g - \beta(V_b - \Delta)$$

The same result can be obtained from the supplementary information of [16].

Inserting $E_D$ given by Eq. (7) into Eq. (3) gives the $G_t$ curves that have been plotted in Fig. 4S(a). As is clear from the plots in Fig. 4S, there are two minima in each $G_t$ spectrum. The primary minimum $V_b^0$ occurs when the Fermi level of the tip is aligned with $E_D$ whereas the secondary minimum $V_b'$ occurs when $E_D$ passes through the Fermi level of graphene.

The position of the primary and the secondary minimum is approximately given by

$$V_b^0 = -\gamma e\,\mathrm{sign}\left(V_g - V_g^D\right)\sqrt{\left|V_g - V_g^D\right|}$$
$$V_b' = \frac{\left(V_g - V_g^0\right)}{\beta} + \Delta \qquad (8)$$

where $V_g^D = V_g^0 - \beta\Delta$ corresponds to the gate voltage at which all the three bands $E_D$, $E_F$ of tip and graphene are aligned. Figs. 4(a,b) show that the above equations correctly predict the positions of the two characteristic minima in each spectrum.

## IV Dirac point mapping

Point to point tunneling spectroscopy, referred to as CITS (Current Imaging Tunneling Spectroscopy), not only gives us the variations of the LDOS as a function of energy but additionally provides a way of directly mapping the spatial variations of the Dirac point. It therefore becomes possible to cross-check if the $G_t(x,y)$ maps acquired at a bias voltage $V_b$ that follows the criterion: $V_b = E_D/e \pm 100$ mV (described in main paper), actually resembles the Dirac point map.

To find the distribution of Dirac point $E_D(\mathbf{r})$ (unperturbed by the tip) from the $G_t$ spectra, as a first step we extract their primary minimum $V_b^0$ (using a parabolic fit over a small energy window of width 350 mV around $V_b^0$). From Eq. (1) of the main manuscript, it is easy to see that at high carrier densities, we have $V_b^0(\mathbf{r}) \approx E_D(\mathbf{r})/e$ while close to charge neutrality, the two quantities start to prominently differ. The CITS measurements presented here have been conducted at high carrier concentrations, so that we can expect the map of $V_b^0$ to mirror the local fluctuations of the Dirac point. Fig. 5S (a) and (d) show the $E_D(\mathbf{r})$ maps obtained at $V_g$ = -15 V (high hole doping, $n_g \approx 4.0 \times 10^{12}$ cm$^{-2}$ ) and 70 V (high electron doping $n_g \approx 3.6 \times 10^{12}$ cm$^{-2}$) respectively of the same region. We can clearly observe the transformation of relatively more strongly hole doped areas in (a) to relatively less electron doped regions in (d), exactly confirming to expectations.

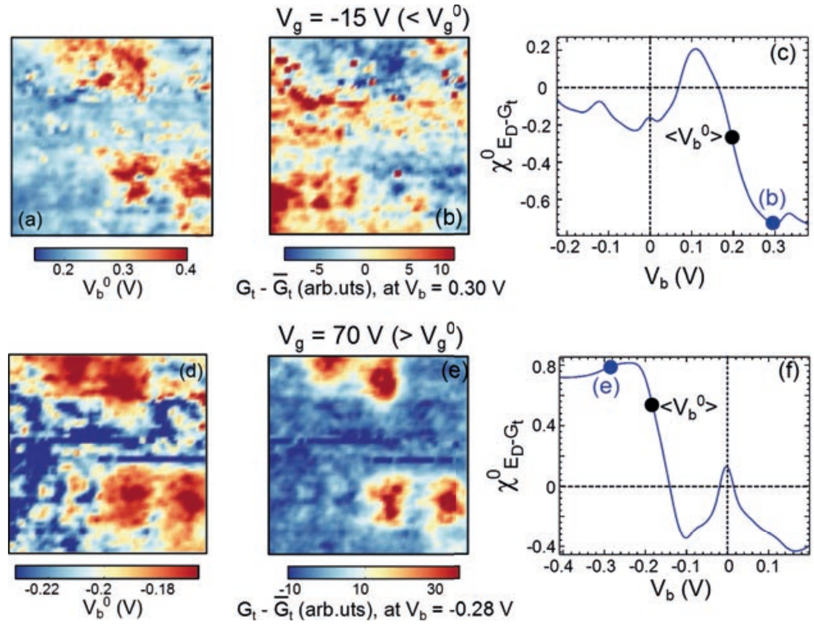


**Fig. 5S**: Experimental demonstration of Dirac point mapping using point to point tunneling spectroscopy at high hole and electron concentrations for a total of 64 x 64 points over an area of 100 x 100 nm$^2$. **(a)-(c)** Extracted from CITS at high hole doping ($V_g$ = -15 V): (a) Spatial map of the fluctuations of the primary minimum $V_b^0$ of the $G_t$ spectrum at each point. **(b)** Map of $(G_t(x,y) - \bar{G})$ at bias $V_b$ = 0.30 V. **(c)** Variation of the 2D correlation coefficient between the maps of $V_b^0$ and $(G_t - \bar{G})$ with bias $V_b$. The black bullet indicates the average $V_b^0$ found in (a); the blue bullet indicates the bias voltage chosen for acquiring (b). **(d)-(f)** Same as in **(a)-(c)** but extracted from CITS at high electron doping ($V_g$ = 70 V).

To compare the $G_t(x,y)$ maps at different $V_b$ with the Dirac point map, we resort to the 2D cross-correlation coefficient between them i.e. $\chi_{ED\text{-}Gt}$ as a function of $V_b$. Fig. 5S (c) and (f) show the variation of $\chi_{ED\text{-}Gt}$ with $V_b$ at the two different $V_g$. At high hole doping, $|\chi_{ED\text{-}Gt}|$ is maximum at $V_b > \bar{E}_D + 0.1$ V which implies a strong resemblance between $G_t(x,y)$ and $E_D(\mathbf{r})$ at these values of $V_b$ which is further proved by the $G_t$ map at $V_b$ = 0.3 V ($=\bar{E}_D + 0.1$ V) in Fig. 5S(b). Similarly, at high electron doping, we observe a maximum correlation at $V_b < \bar{E}_D - 0.1$ V. Hence, this strongly justifies our criteria for selection of $V_b$ for imaging of the doping inhomogeneities at different back-gate voltages.

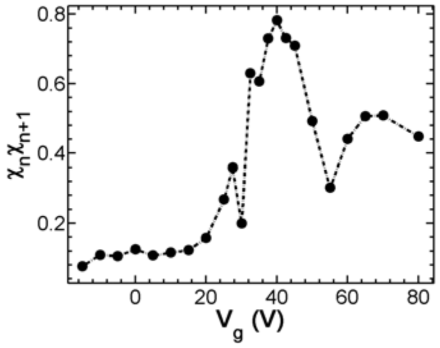


**Fig. 6S:** Local correlation coefficient between two Dirac point maps at two consecutive gate voltages.

We have further analyzed the correlation between Dirac point maps at consecutive gate voltages. The associated local cross-correlation coefficient between $E_D(x,y,V_g)$ and $E_D(x,y,V_G+\delta V_g)$ is shown in Fig. 6S. It is strongest at the Dirac point, where it reaches about 0.8

and decays with increasing doping. This means that at the highest hole doping levels, the puddle maps eventually approach the noise floor, which we situate at ≈ 0.05 in Fig. 6S.

## VI Extraction of Correlation Length

The $G_t$ maps are filtered using a Gaussian filter with FWHM of about 0.55nm, that is, still less than the smallest features we wish to resolve. Next, we find the auto-correlation matrix of $G_t - \langle G_t \rangle$

$$C(\mathrm{i},\mathrm{j}) = \frac{\sum_{m=1}^{M}\sum_{n=1}^{N}\left[G_t(m,n)-\langle G_t\rangle\right]\left[G_t(m+i,n+j)-\langle G_t\rangle\right]}{M\times N} \quad . \qquad (9)$$

Dividing C(i,j) by the central element, $C(0)$, gives the normalized auto-correlation matrix $A(r,\varphi) = C(r,\varphi)/C(0)$. Fig. 7Sb shows a cut in this matrix $A(r,\varphi)$ along a fixed direction $\varphi$. Fitting this curve with a Gaussian function, $G(r) = e^{-r^2/2\xi^2}$ (indicated by the red line in (c)), gives the decay length $\xi$ of the correlation curve for this direction. Repeating this process over all directions and taking the mean gives the angular averaged, normalized correlation function A(r). The angular average of $\xi$ gives the decay length of the correlation curve. This correlation length $\xi$ characterizes the lateral scale of the charge puddles.

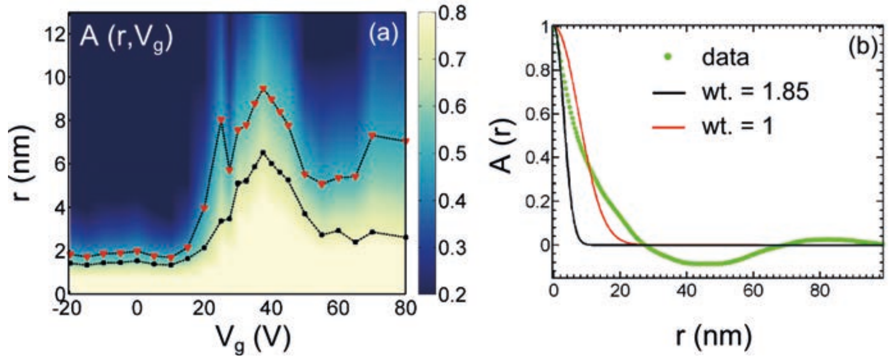


**Fig. 7S: (a)** Color rendering of the angular averaged, normalised auto-correlation $A$ of the charge puddle maps shown in Fig.2 of main text, as a function of distance $r$ and back-gate $V_g$. The red triangles denote correlation length $\xi$ extracted (from Gaussian fit) by applying equal weightage to all data points while black squares denote $\xi$ extracted by applying a relatively higher weightage (weight = 1.85) to data points in the beginning (first 15 nm). **(b)** A(r) corresponding to $G_t(x,y)$ map at $V_g$ = 70 V together with Gaussian fits with equal and increased weightage of the start and end points.

We note here that $\xi$ extracted in this manner is subject to an error due to the finite size of the puddles in comparison to the total size of the image. The larger the size of the puddles, the greater the error, as is the case close to the Dirac point. Additionally, A(r) shows a more pronounced non-Gaussian behavior as charge neutrality is approached, which besides being a finite size effect, is also a characteristic of the correlation function of the screened Coulomb potential. For the sake of comparison with theory, we still use a Gaussian fit to describe the decay of the correlation curves, but associating an error to the extracted $\xi$. In the color plot in Fig. 7S (a), this visually corresponds to the length over which the yellow color (strong correlation) gradually decays into the blue background (vanishing correlation). To determine the error, we perform a Gaussian fit to A(r) with variable weightage of the low r / large data. The difference between the correlation length extracted from these two fits is considered as the error in $\xi$.

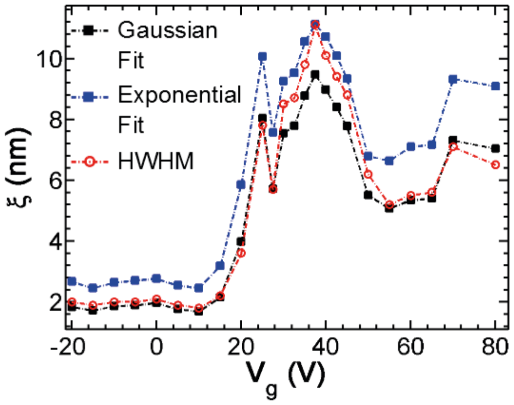


**Fig. 8S:** Puddles size extracted by different methods.

Other procedures can also be adopted to quantify the decay length, such as found from an exponential fit or the half-width at half maximum (Fig. 8(b)). We find that all approaches lead to correlation lengths that differ only slightly. In our analysis, we have used a Gaussian-like decay to fit both the theoretical as well as the experimental correlation curves.

## VI Complementary data at other locations

The growth of the size of the charge puddles close to charge neutrality has been verified at multiple locations on the same single-layered graphene device. At every location investigated, we find an increase both in the lateral scale and amplitude of inhomogeneities. The gate voltage $V_g^D$ at which the maximum inhomogeneity is achieved differs from the overall charge neutrality point of $V_g^0$ = 29 V observed in transport. $V_g^D$ is sometimes found to also slightly change in time, because the work-function mismatch between the tip and the sample can vary in the course of a scanning probe experiment [16].

Fig. 9S shows the measurement of charge puddles at a series of values of $V_g$ at a different location than the one presented in the main text. The charge puddles are seen to gradually grow in size and reaches a maximum at $V_g^D$ = 35 V in this case as is clearly seen from the variation in the $G_t$ maps of the amplitude of the fluctuations ($\delta G_t$) and characteristic size ξ with $V_g$ (Fig. 9S(g,h)). For the amplitude of charge disorder ($\propto \delta G_t$), we find the same relative change between high and low average doping at the different locations. The correlation length ξ, once again, shows good agreement with theoretical predictions based on the parameters ($n_i$, d) extracted from transport.

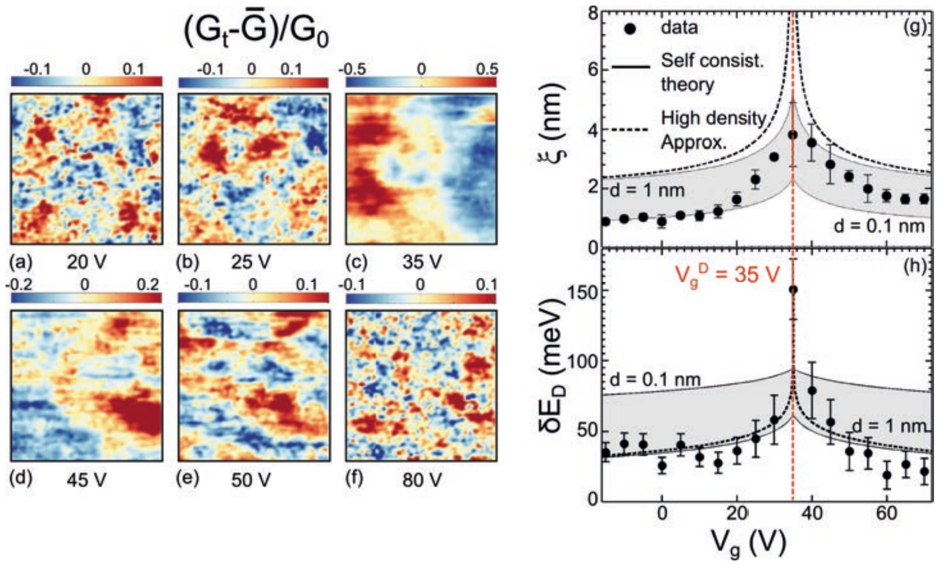


**Fig. 9S: (a)-(f)** Charge puddle maps (or LDOS maps) on graphene at different gate voltages (indicated below each figure) at a different location (Loc. 2) than presented in the main paper (Loc. 1). Area presented is 40 x 40 nm$^2$. The imaging parameters are a modulating voltage of amplitude $V_{AC}$ = 6 mV and frequency f = 322.4 Hz and set-point current $I_t$ = 100 pA at bias voltage $V_b$ equal to **(a)** 0.212 V, **(b)** 0.202 V **(c)** -0.127 V **(d)** -0.127 V **(e)** -0.132 V **(f)** -0.256 V. **(g)** Variation of correlation length ξ and **(h)** standard deviation of Dirac point fluctuations with $V_g$ at Loc.2. The black solid lines represent simulations using self-consistent screening theory for d = 1 nm and 0.1 nm while the black dashed line have been generated without incorporating self-consistent correction to carrier density for d = 1 nm.

## References


[1] K. Nagashio et al., Electrical transport properties of graphene on $SiO_2$ with specific surface structures, *Jour. of Appl. Phys.* **110**, 024513 (2011).
[2] A. C. Ferrari et al., Raman spectrum of graphene and graphene layers, *Phys. Rev. Lett.* **97**, 187401 (2006).
[3] J. Yan et al., Electric field effect tuning of electron-phonon coupling in graphene. *Phys. Rev. Lett.* **98**, 166802 (2007).
[4] A. Das et al., Monitoring dopants by Raman scattering in an electrochemically top-gated graphene transistor, *Nat. Nanotech.* **3**, 210 (2008).
[5] W. Zhu et al., Carrier scattering, mobilities, and electrostatic potential in monolayer, bilayer and trilayer graphene, *Phys. Rev. B* **80**, 235402 (2009).
[6] E. J. H. Lee et al., Contact and edge effects in graphene devices, *Nat. Nanotech.* **3**, 486 (2008).
[7] B. Huard et al., Evidence of the role of contacts on the observed electron-hole asymmetry in graphene, *Phys. Rev. B* **78**, 121402(R) (2008).
[8] D. S. Novikov, Numbers of donors and acceptors from transport measurements in graphene, *Appl. Phys. Lett.* **91**, 102102 (2007).
[9] S. Adam et al., A self-consistent theory for graphene transport, *PNAS* **104**, 18392 (2007).
[10] E. Rossi et al., Effective medium theory for disordered two-dimensional graphene, Phys. Rev. B **79**, 245423 (2009).
[11] Y. W. Tan et al., Measurement of Scattering Rate and Minimum Conductivity in Graphene, *Phys. Rev. Lett.* **99**, 24 (2007).
[12] S. K. Choudhary et al., Effects of tip induced carrier density in local tunnel spectra of graphene, *Appl. Phys. Lett.* **98**, 102109 (2011).
[13] A. H. Castro Neto et al., The electronic properties of graphene, *Rev. Mod. Phys.* **81**, 109 (2009).
[14] S Jung et al., Evolution of microscopic localization in graphene in a magnetic field from scattering resonances to quantum dots, *Nature Phys*. **7**, 245 (2011).
[15] Y-J Yu et al., Tuning the Graphene Work Function by Electric Field Effect, *Nano Lett.* **9**, 3430 (2009)
[16] Y. Zhao et al., Creating and probing electron whispering-gallery modes in graphene, *Science* **348**, 672 (2015).
